# Supplementary material for: Distributed Proximal Gradient Algorithm for Partially Asynchronous Computer Clusters
Source: arXiv:1704.03540 source file (2017-04-11)
Supplement: Supplementary file 1 [file appendix.tex]

%!TEX root = main.tex

%\onecolumn
%{\centering\Large \textbf{Supplementary Materials}}
%\section{Proof of \Cref{thm:example}}\label{sec: example}

%\section{Proof of \Cref{lemma: delay_term_bound}}\label{sec: lemma: delay_term_bound}
